# Supplementary material for: Analytic approach for the number statistics of non-Hermitian random matrices
Source: arXiv:2007.10526 ancillary file (2020-07-20)
Supplement: Supplementary file 1 [file Supplemental.pdf]

# Supplemental Information: Analytic approach for the number statistics of non-Hermitian random matrices

Antonio Tonatiúh Ramos Sánchez
*Department of Quantum Physics and Photonics, Institute of Physics, UNAM, P.O. Box 20-364, 01000 Mexico City, Mexico*

Edgar Guzmán-González and Isaac Pérez Castillo
*Department of Quantum Physics and Photonics, Institute of Physics, UNAM, P.O. Box 20-364, 01000 Mexico City, Mexico and London Mathematical Laboratory, 18 Margravine Gardens, London W6 8RH, United Kingdom*

Fernando L. Metz
*Physics Institute, Federal University of Rio Grande do Sul, 91501-970 Porto Alegre, Brazil and London Mathematical Laboratory, 18 Margravine Gardens, London W6 8RH, United Kingdom*

## PRELIMINARIES

In this supplemental material we present the derivations involved in obtaining an expression for the *cumulant generating function* (CGF) of $\mathcal{N}_{\boldsymbol{A}}(\gamma)$. The sparse random matrix $\boldsymbol{A}$ corresponds with the adjacency matrix of a Poisson random graph with asymmetric edges, as defined in the main text (see Eq. (16)). Given an $N \times N$ non-Hermitian matrix with spectrum $\{\lambda_1, ..., \lambda_N\}$, we introduce the spectral density

$$\rho_{\boldsymbol{A}}(x, y) = N^{-1} \sum_{i=1}^{N} \delta(x - \mathrm{Re}\lambda_i)\, \delta(y - \mathrm{Im}\lambda_i)\ . \tag{1}$$

Then, the number of eigenvalues $\mathcal{N}_{\boldsymbol{A}}(\gamma)$ within a region $D \subset \mathbb{C}$, enclosed by a contour $\gamma = \partial D$, is given by

$$\mathcal{N}_{\boldsymbol{A}}(\gamma) = N \int_D dxdy\, \rho_{\boldsymbol{A}}(x, y)\ . \tag{2}$$

If $\boldsymbol{A}$ is a random matrix drawn from a distribution $\mathcal{P}(\boldsymbol{A})$, then the CGF of $\mathcal{N}_{\boldsymbol{A}}(\gamma)$ is defined as

$$\mathcal{F}_\gamma(\mu) = -\lim_{N\to\infty} \frac{1}{N} \ln \left\langle e^{-\mu \mathcal{N}_{\boldsymbol{A}}(\gamma)} \right\rangle , \tag{3}$$

where $\langle \cdots \rangle$ denotes the average over the distribution $\mathcal{P}(\boldsymbol{A})$. The first step to compute the ensemble average of Eq. (3) consists in understanding how $\mathcal{N}_{\boldsymbol{A}}$ depends on $\boldsymbol{A}$. To achieve this, we rewrite the spectral density as

$$\rho_{\boldsymbol{A}}(x, y) = \frac{1}{N\pi} \partial_z \partial_{z^*} \ln\det\left[(z\boldsymbol{I}_N - \boldsymbol{A})(z\boldsymbol{I}_N - \boldsymbol{A})^\dagger\right] , \tag{4}$$

with $\partial_z = 2^{-1}(\partial_x - i\partial_y)$, $\partial_{z^*} = (2i)^{-1}(\partial_x + i\partial_y)$ and $\boldsymbol{I}_N$ being the $N \times N$ identity matrix. Substituting Eq. (4) in Eq. (2) and applying Stokes' theorem yields

$$\mathcal{N}_{\boldsymbol{A}}(\gamma) = -\oint_\gamma \frac{dz}{2\pi i} \partial_z \ln Q_{\boldsymbol{A}}(z, z^*)\ , \tag{5}$$

where we have introduced

$$Q_{\boldsymbol{A}}(z, z^*) = \frac{1}{\det\left[(\boldsymbol{A} - z\boldsymbol{I}_N)(\boldsymbol{A} - z\boldsymbol{I}_N)^\dagger\right]}\ . \tag{6}$$

## THE REPLICA APPROACH

Having established the basic concepts of the derivation, we will rewrite Eq. (6) in a more suitable form. We first discretize the contour integral along $\gamma$ by introducing a set of points $z_1, ..., z_L$ such that $z_{L+1} = z_1$ and $z_{l+1} = z_l + \Delta z_l$ for all $l$. Eqs. (5) and

(3) can be reformulated as

$$\mathcal{N}_{\boldsymbol{A}}(\gamma) = -\frac{1}{2\pi i}\lim_{L\to\infty}\sum_{l=1}^{L}\left[\ln Q_{\boldsymbol{A}}\left(z_{l+1}, z_l^*\right) - \ln Q_{\boldsymbol{A}}\left(z_l, z_l^*\right)\right] , \tag{7}$$

and

$$\mathcal{F}_{\gamma}(\mu) = -\lim_{N\to\infty}\frac{1}{N}\lim_{L\to\infty}\lim_{n_\pm\to\pm\frac{\mu}{2\pi i}}\ln\left\langle\prod_{l=1}^{L}\left[Q_{\boldsymbol{A}}\left(z_{l+1}, z_l^*\right)\right]^{n_+}\left[Q_{\boldsymbol{A}}\left(z_l, z_l^*\right)\right]^{n_-}\right\rangle , \tag{8}$$

respectively. The next step is to express $Q_{\boldsymbol{A}}$ as a multivariate Gaussian integral. We first introduce the block matrix

$$\boldsymbol{F}_{\eta}\left(z, z^*\right) = \begin{pmatrix} \eta\boldsymbol{I}_N & i\left(z\boldsymbol{I}_N - \boldsymbol{A}\right) \\ i\left(z\boldsymbol{I}_N - \boldsymbol{A}\right)^{\dagger} & \eta\boldsymbol{I}_N \end{pmatrix} , \tag{9}$$

which is related to $Q_{\boldsymbol{A}}$ via $Q_{\boldsymbol{A}}(z, z^*) = \lim_{\eta\to 0^+}\left(\det\boldsymbol{F}_{\eta}(z, z^*)\right)^{-1}$. The parameter $\eta > 0$ simply ensures that $\boldsymbol{F}_{\eta}$ has a positive Hermitian part, thus allowing us to represent $Q_{\boldsymbol{A}}$ as a multivariate Gaussian integral over a set of spinors $\psi_i \in \mathbb{C}^2$, $i = 1, ..., N$,

$$Q_{\boldsymbol{A}}\left(z, z^*\right) = \lim_{\eta\to 0^+}\int\left[\prod_{i=1}^{N}\frac{d\psi_i d\psi_i^{\dagger}}{\pi^2}\right]\exp\left[-\sum_{i=1}^{N}\psi_i^{\dagger}\boldsymbol{M}_{\eta}\left(z, z^*\right)\psi_i + i\sum_{i,j=1}^{N}\psi_i^{\dagger}\boldsymbol{B}_{ij}\psi_j\right] , \tag{10}$$

with

$$\boldsymbol{M}_{\eta}(z, z^*) = \eta\boldsymbol{I}_2 + i\left(z\boldsymbol{\sigma}_+ + z^*\boldsymbol{\sigma}_-\right) , \qquad \boldsymbol{B}_{ij} = A_{ij}\boldsymbol{\sigma}_+ + A_{ij}^{\dagger}\boldsymbol{\sigma}_- , \tag{11}$$

and $\boldsymbol{\sigma}_+$, $\boldsymbol{\sigma}_-$ are the usual ladder operators

$$\boldsymbol{\sigma}_+ = \begin{pmatrix} 0 & 1 \\ 0 & 0 \end{pmatrix} , \qquad \boldsymbol{\sigma}_- = \begin{pmatrix} 0 & 0 \\ 1 & 0 \end{pmatrix} . \tag{12}$$

Since $\psi_i = (u_i, v_i)^T$ is a spinor with components $u_i, v_i \in \mathbb{C}^2$, the measure $d\psi_i d\psi_i^{\dagger}$ is given by

$$\frac{d\psi_i d\psi_i^{\dagger}}{\pi^2} = \frac{d\mathrm{Re}u_i d\mathrm{Im}u_i}{\pi}\frac{d\mathrm{Re}v_i d\mathrm{Im}v_i}{\pi} . \tag{13}$$

We will also write $d\Psi_i \equiv d\psi_i d\psi_i^{\dagger}/\pi^2$ in order to shorten the notation. Following the main strategy of the replica approach and assuming that $n_\pm$ are positive integers in Eq. (8), we can rewrite this expression as follows

$$\begin{aligned} e^{-N\mathcal{F}_{\gamma}(\mu)} = &\int\left[\prod_{i=1}^{N}\prod_{l=1}^{L}\prod_{a=1}^{n_+}d\Psi_{i,la}\right]\left[\prod_{i=1}^{N}\prod_{l=1}^{L}\prod_{b=1}^{n_-}d\Phi_{i,lb}\right] \\ &\times\exp\left[-\sum_{i=1}^{N}\sum_{l=1}^{L}\left(\sum_{a=1}^{n_+}\psi_{i,la}^{\dagger}\boldsymbol{M}_{\eta}(z_{l+1}, z_l^*)\psi_{i,la} + \sum_{b=1}^{n_-}\phi_{i,lb}^{\dagger}\boldsymbol{M}_{\eta}(z_l, z_l^*)\phi_{i,lb}\right)\right] \\ &\times\left\langle\exp\left[i\sum_{i<j}^{N}\sum_{l=1}^{L}\left\{\sum_{a=1}^{n_+}\left(\psi_{i,la}^{\dagger}\boldsymbol{B}_{ij}\psi_{j,la} + \psi_{j,la}^{\dagger}\boldsymbol{B}_{ij}^{\dagger}\psi_{i,la}\right) + \sum_{b=1}^{n_-}\left(\phi_{i,lb}^{\dagger}\boldsymbol{B}_{ij}\phi_{j,lb} + \phi_{j,lb}^{\dagger}\boldsymbol{B}_{ij}^{\dagger}\phi_{i,lb}\right)\right\}\right]\right\rangle , \end{aligned} \tag{14}$$

where, for simplicity, we have set $A_{ii} = 0$. We have also assumed that the limits appearing in Eq. (8) are implicit. The next step is to calculate the average over the distribution of $\boldsymbol{A}$. Thus, we must consider a particular form for the ensemble of random matrices. Here we will present results for the adjacency matrix $\boldsymbol{A}$ of weighted Poisson graphs with asymmetric edges, where the matrix elements are defined as $A_{ij} = c_{ij}J_{ij}$, and $\{c_{ij}\}_{i,j=1,...,N}$ are drawn from the distribution

$$p_c(\{c_{ij}\}) = \prod_{i<j}\left[\frac{c}{N}\delta_{c_{ij},1} + \left(1 - \frac{c}{N}\right)\delta_{c_{ij},0}\right] ,$$

with $c_{ij} = c_{ji}$ and $c_{ii} = 0$. The number of links connected to an arbitrary node follows a Poisson distribution with average $c \in \mathbb{R}^+$. The binary random variables $\{c_{ij}\}_{i,j=1,\dots,N}$ tell who is connected to whom in the graph, while the real-valued variables $\{J_{ij}\}_{i,j=1,\dots,N}$ control the strength of the pairwise interactions among different sites. These random variables are independently drawn from a distribution $p_J$, so that the weights of the directed links $i \to j$ and $j \to i$ are different, and the random matrix $\boldsymbol{A}$ is asymmetric. After carrying out the average over $\boldsymbol{A}$, we obtain the following expression for $N \gg 1$

$$
\begin{aligned}
e^{-N\mathcal{F}_\gamma(\mu)} = & \int \left[\prod_{i=1}^{N}\prod_{l=1}^{L}\prod_{a=1}^{n_+} d\Psi_{i,la}\right]\left[\prod_{i=1}^{N}\prod_{l=1}^{L}\prod_{b=1}^{n_-} d\Phi_{i,lb}\right] \\
& \times \exp\left[-\sum_{i=1}^{N}\sum_{l=1}^{L}\left(\sum_{a_l=1}^{n_+}\psi_{i,a_l}^\dagger \boldsymbol{M}_\eta(z_{l+1}, z_l^*)\psi_{i,a_l} + \sum_{b=1}^{n_-}\phi_{i,lb}^\dagger \boldsymbol{M}_\eta(z_l, z_l^*)\phi_{i,lb}\right)\right] \\
& \times \exp\left[\frac{c}{2N}\sum_{i,j=1}^{N}\left\langle \exp\left[i\sum_{l=1}^{L}\left\{\sum_{a=1}^{n_+}\left(\psi_{i,la}^\dagger \boldsymbol{J}\psi_{j,la} + \psi_{j,la}^\dagger \boldsymbol{J}^\dagger\psi_{i,la}\right) + \sum_{b=1}^{n_-}\left(\phi_{i,lb}^\dagger \boldsymbol{J}\phi_{j,lb} + \phi_{j,lb}^\dagger \boldsymbol{J}^\dagger\phi_{i,lb}\right)\right\}\right] - 1\right\rangle_{\boldsymbol{J}}\right],
\end{aligned}
\tag{15}
$$

where $\langle(\cdots)\rangle_{\boldsymbol{J}}$ stands for the average over

$$
\boldsymbol{J} = J\boldsymbol{\sigma}_+ + J'\boldsymbol{\sigma}_-, \tag{16}
$$

with the random interactions $J$ and $J'$ independently drawn from $p_J$.

Next, in order to decouple sites, we introduce the following order-parameter function

$$
P(\boldsymbol{\Psi}, \boldsymbol{\Phi}) \equiv P(\boldsymbol{\Psi}, \boldsymbol{\Phi}; \{\boldsymbol{\Psi}_i, \boldsymbol{\Phi}_i\}_{i=1}^N) = \frac{1}{N}\sum_{i=1}^{N}\prod_{l=1}^{L}\left[\prod_{a=1}^{n_+}\delta(\psi_{la} - \psi_{i,la})\right]\left[\prod_{b=1}^{n_-}\delta(\phi_{lb} - \phi_{i,lb})\right], \tag{17}
$$

where we have introduced the shorthand notations $\boldsymbol{\Psi} = \{\psi_{la}\}$ and $\boldsymbol{\Phi} = \{\phi_{lb}\}$, for $l = 1, \dots, L$, $a = 1, \dots, n_+$ and $b = 1, \dots, n_-$. Analogously, we have also defined $\boldsymbol{\Psi}_i \equiv \{\psi_{i,la}\}$ and $\boldsymbol{\Phi}_i \equiv \{\psi_{i,la}\}$, with $i = 1, \dots, N$. After some tedious algebra, we can write $e^{-N\mathcal{F}_\gamma(\mu)}$ as the following path integral over $P(\boldsymbol{\Psi}, \boldsymbol{\Phi})$ and the conjugate order-parameter $\hat{P}(\boldsymbol{\Psi}, \boldsymbol{\Phi})$

$$
e^{-N\mathcal{F}_\gamma(\mu)} = \int \mathcal{D}[\{P, \hat{P}\}] e^{-NS\left[\{P, \hat{P}\}\right]}, \tag{18}
$$

where $S\left[\left\{P, \hat{P}\right\}\right]$ is defined as follows

$$
\begin{aligned}
S\left[\left\{P, \hat{P}\right\}\right] = & -\ln\left\{\int d\boldsymbol{\Psi} d\boldsymbol{\Phi} \exp\left[-\sum_{l=1}^{L}\left(\sum_{a=1}^{n_+}\psi_{a_l}^\dagger \boldsymbol{M}(z_{l+1}, z_l^*)\psi_{a_l} + \sum_{b=1}^{n_-}\phi_{b_l}^\dagger \boldsymbol{M}(z_l, z_l^*)\phi_{b_l}\right) - i\hat{P}(\boldsymbol{\Psi}, \boldsymbol{\Phi})\right]\right\} \\
& - \frac{c}{2}\int d\boldsymbol{\Psi} d\boldsymbol{\Psi}' d\boldsymbol{\Phi} d\boldsymbol{\Phi}' P(\boldsymbol{\Psi}, \boldsymbol{\Phi}) P(\boldsymbol{\Psi}', \boldsymbol{\Phi}') \left\langle e^{i\sum_{l=1}^{L}\left\{\sum_{a=1}^{n_+}\left[\psi_{la}^\dagger \boldsymbol{J}\psi'_{la} + (\psi'_{la})^\dagger \boldsymbol{J}^\dagger\psi_{la}\right] + \sum_{b=1}^{n_-}\left[\phi_{lb}^\dagger \boldsymbol{J}\phi'_{lb} + (\phi'_{lb})^\dagger \boldsymbol{J}^\dagger\phi_{lb}\right]\right\}} - 1\right\rangle_{\boldsymbol{J}} \\
& - i\int d\boldsymbol{\Psi} d\boldsymbol{\Phi} P(\boldsymbol{\Psi}, \boldsymbol{\Phi}) \hat{P}(\boldsymbol{\Psi}, \boldsymbol{\Phi}) .
\end{aligned}
\tag{19}
$$

**The saddle-point method and the replica symmetric ansatz**

Using the saddle-point method, the integral in Eq. (18) is solved in the limit $N \to \infty$, resulting in $\int \mathcal{D}[\{P, \hat{P}\}] e^{-NS\left[\{P, \hat{P}\}\right]} \asymp e^{-NS\left[\{P_0, \hat{P}_0\}\right]}$, where $P_0, \hat{P}_0$ are a pair of functions that extremize the functional $S\left[\left\{P, \hat{P}\right\}\right]$. Thus they obey the following saddle-point equations

$$
-i\hat{P}(\boldsymbol{\Psi}, \boldsymbol{\Phi}) = c\int d\boldsymbol{\Psi} d\boldsymbol{\Phi} P(\boldsymbol{\Psi}', \boldsymbol{\Phi}') \left\langle e^{i\sum_{l=1}^{L}\left\{\sum_{a=1}^{n_+}\left(\psi_{la}^\dagger \boldsymbol{J}\psi'_{la} + (\psi'_{la})^\dagger \boldsymbol{J}^\dagger\psi_{la}\right) + \sum_{b=1}^{n_-}\left(\phi_{lb}^\dagger \boldsymbol{J}\phi'_{lb} + )\phi'_{lb})^\dagger \boldsymbol{J}^\dagger\phi_{lb}\right)\right\}} - 1\right\rangle_{\boldsymbol{J}}, \tag{20}
$$

$$
P(\boldsymbol{\Psi}, \boldsymbol{\Phi}) = \frac{\exp\left[-\sum_{l=1}^{L}\left(\sum_{a=1}^{n_+}\psi_{la}^\dagger \boldsymbol{M}_\eta(z_{l+1}, z_l^*)\psi_{la} + \sum_{b=1}^{n_-}\phi_{lb}^\dagger \boldsymbol{M}_\eta(z_l, z_l^*)\phi_{lb}\right) - i\hat{P}(\boldsymbol{\Psi}, \boldsymbol{\Phi})\right]}{\int d\boldsymbol{\Psi}' d\boldsymbol{\Phi}' \exp\left[-\sum_{l=1}^{L}\left(\sum_{a=1}^{n_+}\psi'^\dagger_{la} \boldsymbol{M}_\eta(z_{l+1}, z_l^*)\psi'_{la} + \sum_{b=1}^{n_-}\phi'^\dagger_{lb} \boldsymbol{M}_\eta(z_l, z_l^*)\phi'_{lb}\right) - i\hat{P}(\boldsymbol{\Psi}', \boldsymbol{\Phi}')\right]}, \tag{21}
$$

where, for simplicity, we have dropped the subindex zero. To push further the derivation, we assume the replica symmetric (RS) ansatz

$$P\left(\mathbf{\Psi},\mathbf{\Phi}\right)=\int\left[\prod_{l=1}^{L}d\mathbf{\Sigma}_l d\mathbf{\Gamma}_l\right]\omega\left(\{\mathbf{\Sigma}_l,\mathbf{\Gamma}_l\}_{l=1}^{L}\right)\prod_{l=1}^{L}\left[\prod_{a=1}^{n_+}\frac{e^{-\psi_{la}^{\dagger}\mathbf{\Sigma}_l^{-1}\psi_{la}}}{\det\mathbf{\Sigma}_l}\prod_{b=1}^{n_-}\frac{e^{-\phi_{lb}^{\dagger}\mathbf{\Gamma}_l^{-1}\phi_{lb}}}{\det\mathbf{\Gamma}_l}\right], \tag{22}$$

where $\mathbf{\Sigma}_l$ and $\mathbf{\Gamma}_l$ are $2\times 2$ complex matrices defined for each $z_l\in\gamma$, and $\omega\left(\{\mathbf{\Sigma}_l,\mathbf{\Gamma}_l\}_{l=1}^{L}\right)$ is the joint probability distribution of the pairs of matrices $\{\mathbf{\Sigma}_l,\mathbf{\Gamma}_l\}_{l=1}^{L}$ along the $L$ points on the contour.

Combining Eqs. (20) and (21) in a single equation for $P\left(\mathbf{\Psi},\mathbf{\Phi}\right)$, expanding its numerator in powers of $c$, using the RS ansatz (22), and resolving the various integrals, we obtain the following self-consistency equation for $\omega\left(\{\mathbf{\Sigma}_l,\mathbf{\Gamma}_l\}_{l=1}^{L}\right)$

$$\begin{aligned}\omega\left(\{\mathbf{\Sigma}_l,\mathbf{\Gamma}_l\}_{l=1}^{L}\right)=&\frac{1}{\Lambda}\sum_{k=0}^{\infty}\frac{e^{-c}c^k}{k!}\int\left[\prod_{r=1}^{k}dJ_r\prod_{l=1}^{L}\mathrm{d}\mathbf{\Sigma}_{lr}\mathrm{d}\mathbf{\Gamma}_{lr}\right]\left[\prod_{r=1}^{k}p_J\left(J_r\right)\omega\left(\{\mathbf{\Sigma}_{lr},\mathbf{\Gamma}_{lr}\}_{l=1}^{L}\right)\right]\\&\times\exp\left[-\frac{\mu}{2\pi i}\sum_{l=1}^{L}\ln\det\left(\boldsymbol{M}_\eta\left(z_{l+1},z_l^*\right)+\sum_{r=1}^{k}\boldsymbol{J}_r\mathbf{\Sigma}_{lr}\boldsymbol{J}_r^{\dagger}\right)+\frac{\mu}{2\pi i}\sum_{l=1}^{L}\ln\det\left(\boldsymbol{M}_\eta\left(z_l,z_l^*\right)+\sum_{r=1}^{k}\boldsymbol{J}_r\mathbf{\Gamma}_{lr}\boldsymbol{J}_r^{\dagger}\right)\right]\\&\times\prod_{l=1}^{L}\delta\left[\mathbf{\Sigma}_l-\frac{1}{\boldsymbol{M}_\eta\left(z_{l+1},z_l^*\right)+\sum_{r=1}^{k}\boldsymbol{J}_r\mathbf{\Sigma}_{lr}\boldsymbol{J}_r^{\dagger}}\right]\prod_{l=1}^{L}\delta\left[\mathbf{\Gamma}_l-\frac{1}{\boldsymbol{M}_\eta\left(z_l,z_l^*\right)+\sum_{r=1}^{k}\boldsymbol{J}_r\mathbf{\Gamma}_{lr}\boldsymbol{J}_r^{\dagger}}\right],\end{aligned} \tag{23}$$

where we have already performed the replica limit $n_\pm\to\pm\frac{\mu}{2\pi i}$. Similarly, we can also obtain an expression for the CGF by evaluating $S\left[\left\{P,\hat{P}\right\}\right]$, given by Eq. (19), at the replica-symmetric saddle-point. Inserting Eq. (22) in Eq. (19) and calculating the remainder integrals, we obtain

$$\begin{aligned}\mathcal{F}_\gamma(\mu)=&-\ln\Bigg\{\sum_{k=0}^{\infty}\frac{e^{-c}c^k}{k!}\int\left[\prod_{r=1}^{k}\mathrm{d}\boldsymbol{J}_r p\left(J_r\right)\right]\left[\prod_{r=1}^{k}\prod_{l=1}^{L}\mathrm{d}\mathbf{\Sigma}_{lr}\mathrm{d}\mathbf{\Gamma}_{lr}\right]\prod_{r=1}^{k}\omega\left(\{\mathbf{\Sigma}_{lr},\mathbf{\Gamma}_{lr}\}_{l=1}^{L}\right)\\&\times\exp\left[-\frac{\mu}{2\pi i}\sum_{l=1}^{L}\ln\det\left(\boldsymbol{M}_\eta\left(z_{l+1},z_l^*\right)+\sum_{r=1}^{k}\boldsymbol{J}_r\mathbf{\Sigma}_{lr}\boldsymbol{J}_r^{\dagger}\right)+\frac{\mu}{2\pi i}\sum_{l=1}^{L}\ln\det\left(\boldsymbol{M}_\eta\left(z_l,z_l^*\right)+\sum_{r=1}^{k}\boldsymbol{J}_r\mathbf{\Gamma}_{lr}\boldsymbol{J}_r^{\dagger}\right)\right]\Bigg\}\\&+\frac{c}{2}\int p_J(J)dJ\int\left[\prod_{l=1}^{L}\mathrm{d}\mathbf{\Sigma}_l d\mathbf{\Gamma}_l d\mathbf{\Sigma}_l' d\mathbf{\Gamma}_l'\right]\omega\left(\{\mathbf{\Sigma}_l,\mathbf{\Gamma}_l\}_{l=1}^{L}\right)\omega\left(\{\mathbf{\Sigma}_l',\mathbf{\Gamma}_l'\}_{l=1}^{L}\right)\\&\times\exp\left[-\frac{\mu}{2\pi i}\sum_{l=1}^{L}\ln\det\left(\boldsymbol{I}_2+\mathbf{\Sigma}_l\boldsymbol{J}\mathbf{\Sigma}_l'\boldsymbol{J}^{\dagger}\right)+\frac{\mu}{2\pi i}\sum_{l=1}^{L}\ln\det\left(\boldsymbol{I}_2+\mathbf{\Gamma}_l\boldsymbol{J}\mathbf{\Gamma}_l'\boldsymbol{J}^{\dagger}\right)\right]-\frac{c}{2}.\end{aligned} \tag{24}$$

The final step is to perform the continuum limit $L\to\infty$.

**The continuous limit along the contour**

Let us now take the continuous limit $L\to\infty$ in Eqs. (23) and (24). From the definition of $\boldsymbol{M}_\eta$, Eq. (11), we obtain that

$$\boldsymbol{M}_\eta\left(z_{l+1},z_l^*\right)=\boldsymbol{M}_\eta\left(z_l,z_l^*\right)+i\Delta z_l\boldsymbol{\sigma}_++\mathcal{O}(\Delta z_l^2), \tag{25}$$

for $\Delta z_l\ll 1$. Henceforth we expand all quantities in powers of $\Delta z_l$ up to the leading term. As a result, we get

$$\left[\boldsymbol{M}_\eta\left(z_{l+1},z_l^*\right)+\sum_{r=1}^{k}\boldsymbol{J}_r\mathbf{\Sigma}_{lr}\boldsymbol{J}_r^{\dagger}\right]^{-1}=\frac{1}{\boldsymbol{M}_\eta\left(z_l,z_l^*\right)+\sum_{r=1}^{k}\boldsymbol{J}_r\mathbf{\Sigma}_{lr}\boldsymbol{J}_r^{\dagger}}\left(\boldsymbol{I}_2-\sigma_+\frac{i\Delta z_l}{\boldsymbol{M}_\eta\left(z_l,z_l^*\right)+\sum_{r=1}^{k}\boldsymbol{J}_r\mathbf{\Sigma}_{lr}\boldsymbol{J}_r^{\dagger}}\right). \tag{26}$$

From the arguments of the Dirac deltas appearing in the self-consistency Eq. (23), we see that it is convenient to make the following change of variables $\mathbf{\Sigma}_l = \mathbf{\Gamma}_l + \Delta z_l \boldsymbol{R}_l$, so that the RHS of Eq. (26) can be rewritten as

$$\begin{aligned}\mathbf{\Gamma}_l + \Delta z_l \boldsymbol{R}_l \leftarrow & \frac{1}{\boldsymbol{M}_\eta\left(z_l, z_l^*\right) + \sum_{r=1}^{k} \boldsymbol{J}_r \mathbf{\Gamma}_{l_r} \boldsymbol{J}_r^\dagger} + \Delta z_l \left[\frac{1}{\boldsymbol{M}_\eta\left(z_l, z_l^*\right) + \sum_{r=1}^{k} \boldsymbol{J}_r \mathbf{\Gamma}_{lr} \boldsymbol{J}_r^\dagger} i\sigma_+ \frac{1}{\boldsymbol{M}_\eta\left(z_l, z_l^*\right) + \sum_{r=1}^{k} \boldsymbol{J}_r \mathbf{\Gamma}_{lr} \boldsymbol{J}_r^\dagger} + \right. \\ & \left. \frac{1}{\boldsymbol{M}_\eta\left(z_l, z_l^*\right) + \sum_{r=1}^{k} \boldsymbol{J}_r \mathbf{\Gamma}_{lr} \boldsymbol{J}_r^\dagger} \sum_{r=1}^{k} \boldsymbol{J}_r \boldsymbol{R}_{lr} \boldsymbol{J}_r^\dagger \frac{1}{\boldsymbol{M}_\eta\left(z_l, z_l^*\right) + \sum_{r=1}^{k} \boldsymbol{J}_r \mathbf{\Gamma}_{lr} \boldsymbol{J}_r^\dagger}\right].\end{aligned} \tag{27}$$

Plugging Eq. (27) into Eqs. (23) and (24) and taking the limit $L \to \infty$, we arrive at the final equations

$$\begin{aligned}\omega\left[\{\boldsymbol{R}, \mathbf{\Gamma}\}\right] = & \frac{1}{\Lambda} \sum_{k=0}^{\infty} \frac{e^{-c} c^k}{k!} \int \left[\prod_{r=1}^{k} d\{\boldsymbol{R}_r, \mathbf{\Gamma}_r\} \omega\left[\{\boldsymbol{R}_r, \mathbf{\Gamma}_r\}\right]\right] e^{\frac{\mu}{2\pi i} \oint_\gamma dz \mathrm{Tr}\left[\boldsymbol{R}(z) \mathbf{\Gamma}^{-1}(z)\right]} \\ & \left\langle \delta_{(\mathrm{F})}\left[\boldsymbol{R} + \mathbf{\Gamma}\left(i\sigma_+ + \sum_{r=1}^{k} \boldsymbol{J}_r \boldsymbol{R}_r \boldsymbol{J}_r^\dagger\right) \mathbf{\Gamma}\right] \delta_{(\mathrm{F})}\left[\mathbf{\Gamma} - \frac{1}{\boldsymbol{M}_\eta + \sum_{r=1}^{k} \boldsymbol{J}_r \mathbf{\Gamma}_r \boldsymbol{J}_r^\dagger}\right]\right\rangle_{\boldsymbol{J}_{1,\ldots,k}}\end{aligned} \tag{28}$$

and

$$\begin{aligned}\mathcal{F}_\gamma(\mu) = & \frac{c}{2} + \frac{c}{2} \int d\left\{\boldsymbol{R}, \mathbf{\Gamma}\right\} d\left\{\boldsymbol{R}', \mathbf{\Gamma}'\right\} \omega\left[\{\boldsymbol{R}, \mathbf{\Gamma}\}\right] \omega\left[\{\boldsymbol{R}', \mathbf{\Gamma}'\}\right] \\ & \times \left\langle \exp\left(-\frac{\mu}{2\pi i} \oint_\gamma dz \mathrm{Tr}\left\{\left[\boldsymbol{I}_2 + \mathbf{\Gamma}(z) \boldsymbol{J} \mathbf{\Gamma}'(z) \boldsymbol{J}^\dagger\right]^{-1} \left[\boldsymbol{R}(z) \boldsymbol{J} \mathbf{\Gamma}'(z) \boldsymbol{J}^\dagger + \mathbf{\Gamma}(z) \boldsymbol{J} \boldsymbol{R}'(z) \boldsymbol{J}^\dagger\right]\right\}\right)\right\rangle_{\boldsymbol{J}} \\ & - \ln\left\langle \sum_{k=0}^{\infty} \frac{e^{-c} c^k}{k!} \int \left[\prod_{r=1}^{k} d\left\{\boldsymbol{R}_r, \mathbf{\Gamma}_r\right\} \omega\left[\{\boldsymbol{R}_r, \mathbf{\Gamma}_r\}\right]\right]\right. \\ & \left. \times \exp\left\{-\frac{\mu}{2\pi i} \oint_\gamma \mathrm{d}z \mathrm{Tr}\left[\left(\boldsymbol{M}_\eta\left(z\right) + \sum_{r=1}^{k} \boldsymbol{J}_r \mathbf{\Gamma}_r(z) \boldsymbol{J}_r^\dagger\right)^{-1} \left(i\sigma_+ + \sum_{r=1}^{k} \boldsymbol{J}_r \boldsymbol{R}_r(z) \boldsymbol{J}_r^\dagger\right)\right]\right\}\right\rangle_{\boldsymbol{J}_{1,\ldots,k}},\end{aligned} \tag{29}$$

where $\langle \cdots \rangle_{\boldsymbol{J}_{1,\ldots,k}}$ denotes the average over the $2 \times 2$ matrices $\{\boldsymbol{J}_r\}_{r=1,\ldots,k}$ (see Eq. (16)), $\delta_{(F)}$ represents the Dirac functional delta in the path space, and the path integration measure reads $d\left\{\boldsymbol{R}, \mathbf{\Gamma}\right\} = \lim_{L\to\infty} \prod_{l=1}^{L} d\boldsymbol{R}(z_l) d\mathbf{\Gamma}(z_l)$. The above two equations are the main outcome of our work, since they determine the CGF of the random variable $\mathcal{N}_{\boldsymbol{A}}(\gamma)$ in the limit $N \to \infty$.

## POPULATION DYNAMICS ALGORITHM

Notice that Eq. (28) is a self-consistency equation for the functional probability density $\omega\left[\{\boldsymbol{R}, \mathbf{\Gamma}\}\right]$ along the contour $\gamma$. Here, $\omega\left[\{\boldsymbol{R}, \mathbf{\Gamma}\}\right]$ corresponds to the path density for the pair of matrices $\boldsymbol{R}$ and $\mathbf{\Gamma}$ along $\gamma$ and therefore it contains all possible correlations of these matrices at any collection of points along $\gamma$. Since we are dealing with path integrals, solving numerically Eq. (28) seems a hopeless task. Fortunately, we can adapt the population dynamics algorithm to deal with this situation. The first step consists in discretizing the contour $\gamma$ into a finite number of $L$ points. It is important to realize that this discretization has nothing to do with the original discretization scheme we use to reach the aforementioned equations. Rather, we use a suitable discretization to resolve numerically the contour integrals appearing in the equations for $\omega\left[\{\boldsymbol{R}, \mathbf{\Gamma}\}\right]$ and $\mathcal{F}_\gamma(\mu)$ by seeking an integration algorithm that provides the most efficient quadratures along the contour $\gamma$. Thus, the functional density $\omega\left[\{\boldsymbol{R}, \mathbf{\Gamma}\}\right]$ is replaced by the joint distribution $\omega[\{\boldsymbol{R}(z_l), \mathbf{\Gamma}(z_l)\}_{l=1}^{L}]$. Then we proceed as usual, i.e., we introduce a population with a total number of $M$ matrices $\{\boldsymbol{R}_\alpha(z_1), \ldots, \boldsymbol{R}_\alpha(z_L), \mathbf{\Gamma}_\alpha(z_1), \ldots, \mathbf{\Gamma}_\alpha(z_L)\}_{\alpha=1}^{M}$ at each point $z_l \in \gamma$. The joint distribution $\omega[\{\boldsymbol{R}(z_l), \mathbf{\Gamma}(z_l)\}_{l=1}^{L}]$ is formally given by

$$\omega[\{\boldsymbol{R}(z_l), \mathbf{\Gamma}(z_l)\}_{l=1}^{L}] \sim \frac{1}{M} \sum_{\alpha=1}^{M} \prod_{l=1}^{L} \delta\left[\boldsymbol{R}(z_l) - \boldsymbol{R}_\alpha(z_l)\right] \delta\left[\mathbf{\Gamma}(z_l) - \mathbf{\Gamma}_\alpha(z_l)\right]. \tag{30}$$

Then we use the standard weighted population dynamics algorithm to obtain a numerical solution of Eq. (28), as explained in references [44,46] in the main text. The original path probability density $\omega\left[\{\boldsymbol{R}, \mathbf{\Gamma}\}\right]$ is formally obtained from $\omega[\{\boldsymbol{R}(z_l), \mathbf{\Gamma}(z_l)\}_{l=1}^{L}]$ when $L \to \infty$ and $M \to \infty$.
